# Supplementary material for: Zero-shot Referring Image Segmentation with Global-Local Context Features
Source: arXiv:2303.17811 source file (2023-04-03)
Supplement: Supplementary file 1 [file _supplementary.tex]

\input{_constants}
\cameraready % \review OR \cameraready

\documentclass[10pt,twocolumn,letterpaper]{article}
\input{cvpr_header}
\myexternaldocument{_main}
\begin{document}
%% TITLE
\title{\paperTitle \\ - \textit{Supplementary Materials} -}
\author{\authorBlock}
\maketitle

\input{sections/12_appendix}

{\small
\bibliographystyle{ieee_fullname}
\bibliography{11_references}
}

\end{document}
